# Supplementary material for: Systematically extending classical nucleation theory
Source: arXiv:1804.02920 source file (2018-05-15)
Supplement: Supplementary file 1 [file SI.pdf]

# Supplementary Information for" Beyond Classical Nucleation Theory"

James F. Lutsko
*Center for Nonlinear Phenomena and Complex Systems CP 231,*
*Université Libre de Bruxelles, Blvd. du Triomphe, 1050 Brussels, Belgium*[*]
(Dated: April 9, 2018)

## I. MOVING CLUSTERS

### A. Density

We take the density to be spherically symmetric, but not located at the origin:

$$\rho\left(\mathbf{r};\mathbf{x}\right)=\rho\left(\left|\mathbf{r}-\mathbf{\Delta}\right|;\mathbf{y}\right) \tag{1}$$

where $\mathbf{y}$ are all the parameters besides $\mathbf{\Delta}$. I assume that

$$\frac{\partial}{\partial y^{\alpha}}\rho\left(\left|\mathbf{r}-\mathbf{\Delta}\right|;\mathbf{y}\right) \tag{2}$$

is still spherically symmetric whereas of course,

$$\frac{\partial}{\partial\Delta^{a}}\rho\left(\left|\mathbf{r}-\mathbf{\Delta}\right|;\mathbf{y}\right)=\left(\frac{r^{a}}{r}\frac{\partial\rho\left(r;\mathbf{y}\right)}{\partial r}\right)_{\mathbf{r}=\mathbf{r}-\mathbf{\Delta}}. \tag{3}$$

### B. Poisson Equation

The Poisson equation for the potential for the parameters besides $\mathbf{\Delta}$ will simply be

$$\nabla\cdot\rho\left(\left|\mathbf{r}-\mathbf{\Delta}\right|;\mathbf{x}\right)\nabla\phi_{\alpha}\left(\mathbf{r};\mathbf{x}\right)=\frac{\partial}{\partial y^{\alpha}}\rho\left(\left|\mathbf{r}-\mathbf{\Delta}\right|;\mathbf{y}\right). \tag{4}$$

To solve, we shift the coordinates as

$$\mathbf{r}'=\mathbf{r}-\mathbf{\Delta} \tag{5}$$

and assume that $\phi_{\alpha}\left(\mathbf{r};\mathbf{x}\right)=\phi_{\alpha}\left(\mathbf{r}-\mathbf{\Delta};\mathbf{y}\right)$ so

$$\nabla'\cdot\rho\left(r';\mathbf{y}\right)\nabla'\phi_{\alpha}\left(\mathbf{r}';\mathbf{y}\right)=\frac{\partial\rho\left(r';\mathbf{y}\right)}{\partial y^{\alpha}}. \tag{6}$$

This is solved, in the most general case, by writing

$$\phi_{\alpha}\left(\mathbf{r}';\mathbf{x}\right)=\sum_{l=0}^{\infty}\sum_{m=-l}^{l}f_{lm}\left(r'\right)Y_{lm}\left(\theta',\phi'\right). \tag{7}$$

Substituting into the Poisson equation gives

$$\sum_{l=0}^{\infty}\sum_{m=-l}^{l}\left\{\frac{1}{r'^{2}}\frac{d}{dr'}\rho\left(r';\mathbf{y}\right)r'^{2}\frac{d}{dr'}f_{lm}\left(r'\right)-l\left(l+1\right)\rho\left(r';\mathbf{y}\right)f_{lm}\left(r'\right)\right\}Y_{lm}\left(\theta',\phi'\right)=\frac{\partial\rho\left(r';\mathbf{y}\right)}{\partial y^{\alpha}} \tag{8}$$

---

[*] http://www.lutsko.com

So, multiplying by a spherical harmonic and integrating over the surface and using the completeness of the spherical harmonics gives

$$\frac{1}{r'^2}\frac{d}{dr'}\rho\left(r';\mathbf{y}\right)r'^2\frac{d}{dr'}f_{00}\left(r'\right)=\int\frac{1}{2\sqrt{\pi}}\frac{\partial\rho\left(r';\mathbf{y}\right)}{\partial y^{\alpha}}d\Omega'=2\sqrt{\pi}\frac{\partial\rho\left(r';\mathbf{y}\right)}{\partial y^{\alpha}} \tag{9}$$

and

$$\frac{1}{r'^2}\frac{d}{dr'}\rho\left(r';\mathbf{y}\right)r'^2\frac{d}{dr'}f_{lm}\left(r'\right)-l\left(l+1\right)\rho\left(r';\mathbf{y}\right)f_{lm}\left(r'\right)=0,\ l>0. \tag{10}$$

The first has general solution

$$f_{00}\left(r';\mathbf{y}\right)=A+B\int_{r_0}^{r}\frac{1}{\rho\left(r';\mathbf{y}\right)r'^2}dr'+\frac{2\sqrt{\pi}}{4\pi}\int_{r_0}^{r}\frac{1}{\rho\left(r';\mathbf{y}\right)r'^2}\frac{\partial m\left(r';\mathbf{y}\right)}{\partial y^{\alpha}}dr' \tag{11}$$

and the problem reduces to finding a solution to the second equation. Having done so, we then have that

$$\phi_{\alpha}\left(\mathbf{r};\mathbf{x}\right)=\sum_{l=0}^{\infty}\sum_{m=-l}^{l}f_{lm}\left(\left|\mathbf{r}-\mathbf{\Delta}\right|;\mathbf{y}\right)Y_{lm}\left(\theta',\phi'\right). \tag{12}$$

The no-flux condition becomes

$$\sum_{l=0}^{\infty}\sum_{m=-l}^{l}\left\{\rho\left(\left|\mathbf{r}-\mathbf{\Delta}\right|;\mathbf{y}\right)\frac{\partial}{\partial r}\left[f_{lm}\left(\left|\mathbf{r}-\mathbf{\Delta}\right|;\mathbf{y}\right)Y_{lm}\left(\theta',\phi'\right)\right]\right\}_{R_T}=0. \tag{13}$$

I do not know how to simplify this for the general case. Of course, if $R_T \gg \Delta$ then we would expect that this would basically reduce to

$$\sum_{l=0}^{\infty}\sum_{m=-l}^{l}\rho\left(R_T;\mathbf{y}\right)\left\{\frac{\partial}{\partial r}\left[f_{lm}\left(r;\mathbf{y}\right)\right]\right\}_{R_T}Y_{lm}\left(\theta,\phi\right)=O\left(\Delta/R_T\right). \tag{14}$$

or

$$\left[\frac{\partial}{\partial r}f_{lm}\left(r;\mathbf{y}\right)\right]_{R_T}=O\left(\Delta/R_T\right). \tag{15}$$

If we take, without loss of generality, $\mathbf{\Delta}=\Delta\widehat{\mathbf{z}}$ then

$$\begin{aligned} r' &= \sqrt{r^2-2r\Delta\cos\theta+\Delta^2} \\ \cos\theta' &= \frac{r\cos\theta-\Delta}{\sqrt{r^2-2r\Delta\cos\theta+\Delta^2}} \\ \phi' &= \phi \end{aligned} \tag{16}$$

and

$$\begin{aligned} r &= \sqrt{r'^2+2\Delta r'\cos\theta'+\Delta^2} \\ \cos\theta &= \frac{r'\cos\theta'+\Delta}{\sqrt{r'^2+2\Delta r'\cos\theta'+\Delta^2}} \\ \phi &= \phi' \end{aligned} \tag{17}$$

The spherical surface is

$$\begin{aligned} 0 &= r'^2+2\Delta r'\cos\theta'+\Delta^2-R^2 \\ r &= \sqrt{R^2-\Delta^2\sin^2\theta'}-\Delta\cos\theta' \end{aligned} \tag{18}$$

So

$$\begin{aligned} \frac{\partial}{\partial r} &= \frac{\partial r'}{\partial r}\frac{\partial}{\partial r'}+\frac{\partial\cos\theta'}{\partial r}\frac{\partial}{\partial\cos\theta'} \\ &= \frac{r-\Delta\cos\theta}{r'}\frac{\partial}{\partial r'}+\left(\frac{\cos\theta}{r'}-\frac{\left(r-\Delta\cos\theta\right)\left(r\cos\theta-\Delta\right)}{r'^{3/2}}\right)\frac{\partial}{\partial\cos\theta'} \\ &= \frac{r-\Delta\cos\theta}{r'}\frac{\partial}{\partial r'}+\frac{\Delta\left(1-\cos^2\theta'\right)}{r'\sqrt{r'^2+2\Delta r'\cos\theta'+\Delta^2}}\frac{\partial}{\partial\cos\theta'} \end{aligned} \tag{19}$$

## C. CNT

We take

$$\rho\left(\mathbf{r};\mathbf{y}\right)=\rho_{0}\Theta\left(R-r\right)+\rho_{1}\Theta\left(r-R\right) \tag{20}$$

so

$$\begin{aligned}\frac{\partial}{\partial R}\rho\left(\mathbf{r};\mathbf{y}\right)&=\left(\rho_{0}-\rho_{1}\right)\delta\left(\left|\mathbf{r}-\mathbf{\Delta}\right|-R\right)\\ \frac{\partial}{\partial\Delta}\rho\left(\mathbf{r};\mathbf{y}\right)&=-\left(\rho_{0}-\rho_{1}\right)\delta\left(\left|\mathbf{r}-\mathbf{\Delta}\right|-R\right)\frac{\mathbf{r}-\mathbf{\Delta}}{\left|\mathbf{r}-\mathbf{\Delta}\right|}\end{aligned} \tag{21}$$

so we must solve (in shifted coordinates)

$$\begin{aligned}\nabla'\cdot\rho\left(r';\mathbf{y}\right)\nabla'\phi_{R}\left(\mathbf{r}';\mathbf{y}\right)&=\left(\rho_{0}-\rho_{1}\right)\delta\left(r'-R\right)\\ \nabla'\cdot\rho\left(r';\mathbf{y}\right)\nabla'\phi_{\Delta}\left(\mathbf{r}';\mathbf{y}\right)&=-\left(\rho_{0}-\rho_{1}\right)\delta\left(r'-R\right)\frac{\mathbf{r}'}{r'}\end{aligned} \tag{22}$$

and note that

$$\frac{\mathbf{r}'}{r'}=\left(-\sqrt{\frac{2\pi}{3}}\left(Y_{1}^{-1}+Y_{1}^{1}\right),i\sqrt{\frac{2\pi}{3}}\left(-Y_{1}^{-1}+Y_{1}^{1}\right),\sqrt{\frac{4\pi}{3}}Y_{1}^{0}\right). \tag{23}$$

With the ansatz, we have that

$$\begin{aligned}\sum_{l=0}^{\infty}\sum_{m=-l}^{l}\left\{\frac{1}{r'^{2}}\frac{d}{dr'}\rho\left(r';\mathbf{y}\right)r'^{2}\frac{d}{dr'}f_{lm}^{(R)}\left(r'\right)-\rho\left(r';\mathbf{y}\right)l\left(l+1\right)f_{lm}^{(R)}\left(r'\right)\right\}Y_{lm}\left(\theta',\phi'\right)&=\left(\rho_{0}-\rho_{1}\right)\delta\left(r'-R\right)\\ \sum_{l=0}^{\infty}\sum_{m=-l}^{l}\left\{\frac{1}{r'^{2}}\frac{d}{dr'}\rho\left(r';\mathbf{y}\right)r'^{2}\frac{d}{dr'}f_{lm}^{(\Delta)}\left(r'\right)-\rho\left(r';\mathbf{y}\right)l\left(l+1\right)f_{lm}^{(\Delta)}\left(r'\right)\right\}Y_{lm}\left(\theta',\phi'\right)&=-\left(\rho_{0}-\rho_{1}\right)\delta\left(r'-R\right)\frac{\mathbf{r}'}{r'}\end{aligned} \tag{24}$$

so the only non-trivial components are

$$\begin{aligned}\frac{1}{r'^{2}}\frac{d}{dr'}\rho\left(r';\mathbf{y}\right)r'^{2}\frac{d}{dr'}f_{00}^{(R)}\left(r'\right)&=\left(\rho_{0}-\rho_{1}\right)\delta\left(r'-R\right)\\ \frac{1}{r'^{2}}\frac{d}{dr'}\rho\left(r';\mathbf{y}\right)r'^{2}\frac{d}{dr'}f_{1m}^{(\Delta)}\left(r'\right)-2\frac{1}{r'^{2}}\rho\left(r';\mathbf{y}\right)f_{1m}^{(\Delta)}\left(r'\right)&=-\sqrt{\frac{2\pi}{3}}\left(\rho_{0}-\rho_{1}\right)\delta\left(r'-R\right)\begin{pmatrix}-1&0&-1\\ -i&0&i\\ 0&\sqrt{2}&0\end{pmatrix}\end{aligned} \tag{25}$$

In the two regions inside and outside the boundary,

$$\begin{aligned}\frac{d}{dr'}r'^{2}\frac{d}{dr'}f_{00}^{(R)}\left(r'\right)&=0\\ \frac{d}{dr'}r'^{2}\frac{d}{dr'}f_{1m}^{(\Delta)}\left(r'\right)-2f_{1m}^{(\Delta)}\left(r'\right)&=0\end{aligned} \tag{26}$$

so

$$\begin{aligned}f_{00}^{(R)}\left(r'\right)&=A^{(R)}+\frac{B^{(R)}}{r'}\\ f_{1m}^{(\Delta)}\left(r'\right)&=A^{(R)}r'+\frac{B^{(R)}}{r'^{2}}\end{aligned} \tag{27}$$

and since we need continuity at the border,

$$\begin{aligned}\phi_{R}\left(\mathbf{r}';\mathbf{y}\right)&=\left(A'^{(R)}+\frac{B'^{(R)}}{R}-\frac{B^{(R)}}{R}+\frac{B^{(R)}}{r'}\right)\Theta\left(R-r\right)+\left(A'^{(R)}+\frac{B'^{(R)}}{r'}\right)\Theta\left(r-R\right)\\ \phi_{\Delta}\left(\mathbf{r}';\mathbf{y}\right)&=\left(\left(A_{m}'^{(\Delta)}+\frac{B_{m}'^{(\Delta)}}{R^{3}}-\frac{B_{m}^{(\Delta)}}{R^{3}}\right)r'+\frac{B_{m}^{(\Delta)}}{r'^{2}}\right)Y_{1m}\left(\theta',\phi'\right)\Theta\left(R-r\right)+\left(A_{m}'^{(\Delta)}r'+\frac{B_{m}'^{(\Delta)}}{r'^{2}}\right)Y_{1m}\left(\theta',\phi'\right)\Theta\left(r-R\right)\end{aligned} \tag{28}$$

Completeing the solution requires that

$$\left[\rho_0\left(\frac{B^{(R)}}{R^2}\right)-\rho_1\left(\frac{B'^{(R)}}{R^2}\right)\right]\delta\left(r-R\right)=\left(\rho_0-\rho_1\right)\delta\left(r'-R\right) \tag{29}$$

$$-\rho_0\left(A'^{(\Delta)}_m+\frac{B'^{(\Delta)}_m}{R^3}-\frac{B^{(\Delta)}_m}{R^3}\right)+\rho_1\left(A'^{(\Delta)}_m-2\frac{B'^{(\Delta)}_m}{R^3}\right)=-\sqrt{\frac{2\pi}{3}}\left(\rho_0-\rho_1\right)\begin{pmatrix}-1&0&-1\\-i&0&i\\0&\sqrt{2}&0\end{pmatrix}$$

Supposing that in general $B=0$ to control divergences,

$$B'^{(R)}=-R^2\frac{\rho_0-\rho_1}{\rho_1} \tag{30}$$

$$B'^{(\Delta)}_m=R^3\left(\frac{\rho_0-\rho_1}{\rho_0+2\rho_1}\right)\left(\sqrt{\frac{2\pi}{3}}\begin{pmatrix}-1&0&-1\\-i&0&i\\0&\sqrt{2}&0\end{pmatrix}-A'^{(\Delta)}_m\right)$$

and

$$\phi_R\left(\mathbf{r}';\mathbf{y}\right)=A'^{(R)}-R\frac{\rho_0-\rho_1}{\rho_1}\left[\Theta\left(R-r\right)+\frac{R}{r'}\Theta\left(r-R\right)\right] \tag{31}$$

$$\phi_\Delta\left(\mathbf{r}';\mathbf{y}\right)=A'^{(\Delta)}_m\left\{\left(\frac{3\rho_1}{\rho_0+2\rho_1}\right)r'\Theta\left(R-r\right)+\left(r'+\frac{1}{r'^2}R^3\left(\frac{\rho_1-\rho_0}{\rho_0+2\rho_1}\right)\right)\Theta\left(r-R\right)\right\}Y_{1m}\left(\theta',\phi'\right)$$
$$+\left(\frac{\rho_0-\rho_1}{\rho_0+2\rho_1}\right)\begin{pmatrix}x'\\y'\\z'\end{pmatrix}\left\{\Theta\left(R-r\right)+\left(\frac{R^3}{r'^3}\right)\Theta\left(r-R\right)\right\}$$

Normally, one uses intensivity to demand that $A'^{(\Delta)}_m=0$ giving

$$\phi_R\left(\mathbf{r}';\mathbf{y}\right)=-R\frac{\rho_0-\rho_1}{\rho_1}\left[\Theta\left(R-r'\right)+\frac{R}{r'}\Theta\left(r'-R\right)\right] \tag{32}$$

$$\phi_\Delta\left(\mathbf{r}';\mathbf{y}\right)=\left(\frac{\rho_0-\rho_1}{\rho_0+2\rho_1}\right)\begin{pmatrix}x'\\y'\\z'\end{pmatrix}\left\{\Theta\left(R-r'\right)+\left(\frac{R^3}{r'^3}\right)\Theta\left(r'-R\right)\right\}$$

If there were no shift, no flux would say

$$0=\left[\frac{\partial}{\partial r}\phi_R\left(r;\mathbf{y}\right)\right]_{R_T}=-R\frac{\rho_0-\rho_1}{\rho_1}\left(\frac{R}{R_T}\right) \tag{33}$$

$$0=\left[\frac{\partial}{\partial r}\phi_\Delta\left(\mathbf{r}';\mathbf{y}\right)\right]_{R_T}=A'^{(\Delta)}_m\left\{\left(1-2\left(\frac{R}{R_T}\right)^3\left(\frac{\rho_1-\rho_0}{\rho_0+2\rho_1}\right)\right)\right\}Y_{1m}\left(\theta',\phi'\right)$$
$$+\left(\frac{\rho_0-\rho_1}{\rho_0+2\rho_1}\right)\begin{pmatrix}\widehat{x}\\\widehat{y}\\\widehat{z}\end{pmatrix}\left\{-2\left(\frac{R}{R_T}\right)^3\right\} \tag{34}$$

and neglecting $R/R_T$ leaves $A'^{(\Delta)}_{lm}=0$.

For the general case, we have to add in the homogeneous solution (all orders in $lm$) and then fix coefficients to give no flux on the diplaced surface. Note that in this case the homogeneous solution will be

$$\left(A_{lm}r'^l+\frac{B_{lm}}{r'^{l+1}}\right)Y_{lm}\left(\theta',\phi'\right)\Theta\left(R-r'\right)+\left(A'_{lm}r'^l+\frac{B'_{lm}}{r'^{l+1}}\right)Y_{lm}\left(\theta',\phi'\right)\Theta\left(r'-R\right) \tag{35}$$

and as usual we expect that $B_{lm}=0$ (although it always seems possible that the $l=1$ component could at least be nonzero since the meaure in any integration provides a factor of $r^2$). Continuity at the boundary then gives

$$\left(A'_{lm}+\frac{B'_{lm}}{R^{2l+1}}\right)r'^lY_{lm}\left(\theta',\phi'\right)\Theta\left(R-r'\right)+\left(A'_{lm}r'^l+\frac{B'_{lm}}{r'^{l+1}}\right)Y_{lm}\left(\theta',\phi'\right)\Theta\left(r'-R\right) \tag{36}$$
$$=A'_{lm}r'^lY_{lm}\left(\theta',\phi'\right)+B'_{lm}Y_{lm}\left(\theta',\phi'\right)\frac{1}{R^{l+1}}\left[\left(\frac{r'}{R}\right)^l\Theta\left(R-r'\right)+\left(\frac{R}{r'}\right)^{l+1}\Theta\left(r'-R\right)\right]$$

## II. ELLIPTICAL CLUSTER

### A. Coordinates and geometry

The equation for an ellipsoid is

$$\frac{x^2}{a_1^2}+\frac{y^2}{a_2^2}+\frac{z^2}{a_3^2}=1 \tag{37}$$

and the case $a_1 = a_2 = a_3 = R$ reproduces a sphere. To generalize CNT to this symmetry, we again must solve Laplace's equation in the two regions (inside the cluster and outside) and then apply boundary conditions on the border. The standard approach to this type of problem makes use of confocal ellipsoidal coordinates $(\xi, \mu, \nu)$ defined as the three (real) roots of the equation

$$\frac{x^2}{\lambda^2}+\frac{y^2}{\lambda^2-h_3^2}+\frac{z^2}{\lambda^2-h_2^2}=1 \tag{38}$$

where we define the constants

$$\begin{aligned} h_1^2 &= a_2^2-a_3^2 \\ h_2^2 &= a_1^2-a_3^2 \\ h_3^2 &= a_1^2-a_2^2 \end{aligned} \tag{39}$$

and we are assuming that $0 < a_3 < a_2 < a_{<\infty}$. (Note that Dassios uses $\rho$ rather than $\xi$ but I prefer to avoid confusion with the density by using the latter symbol.) Conventionally, the roots are ordered as

$$0 \le \nu^2 \le h_3^2 \le \mu^2 \le h_2^2 \le \xi^2 \le \infty. \tag{40}$$

The coordinates $\nu$ and $\mu$ take on both positive and negative values while $\xi$ is strictly nonnegative. Explicit formulae for the coordinates are messy but the inverses are easy to express:

$$\begin{aligned} x^2 &= \frac{\xi^2\mu^2\nu^2}{h_2^2h_3^2} \\ y^2 &= \frac{\left(\xi^2-h_3^2\right)\left(\mu^2-h_3^2\right)\left(h_3^2-\nu^2\right)}{h_1^2h_3^2} \\ z^2 &= \frac{\left(\xi^2-h_2^2\right)\left(h_2^2-\mu^2\right)\left(h_2^2-\nu^2\right)}{h_1^2h_2^2}. \end{aligned} \tag{41}$$

Note that the surface defined by $\xi = a_1$, or

$$\begin{aligned} 1 &= \frac{x^2}{a_1^2}+\frac{y^2}{a_1^2-h_3^2}+\frac{z^2}{a_1^2-h_2^2} \\ &= \frac{x^2}{a_1^2}+\frac{y^2}{a_2^2}+\frac{z^2}{a_3^2} \end{aligned} \tag{42}$$

is the ellipsoidal surface of interest. Conversely, if we write the condition for the points inside the ellipsoid of interest,

$$1 > \frac{x^2}{a_1^2}+\frac{y^2}{a_2^2}+\frac{z^2}{a_3^2} \tag{43}$$

and express in terms of ellipsoidal coordinates, we get

$$\begin{aligned} 1 &> \frac{1}{a_1^2}\frac{\xi^2\mu^2\nu^2}{h_2^2h_3^2}+\frac{1}{a_2^2}\frac{\left(\xi^2-h_3^2\right)\left(\mu^2-h_3^2\right)\left(h_3^2-\nu^2\right)}{h_1^2h_3^2}+\frac{1}{a_3^2}\frac{\left(\xi^2-h_2^2\right)\left(h_2^2-\mu^2\right)\left(h_2^2-\nu^2\right)}{h_1^2h_2^2} \\ &> 1+\frac{\left(\xi^2-a_1^2\right)\left(\mu^2-a_1^2\right)\left(\nu^2-a_1^2\right)}{a_1^2a_2^2a_3^2} \end{aligned} \tag{44}$$

giving

$$0 > \frac{\left(\xi^2 - a_1^2\right)\left(\mu^2 - a_1^2\right)\left(\nu^2 - a_1^2\right)}{a_1^2 a_2^2 a_3^2} \tag{45}$$

or

$$0 < \left(a_1^2 - \xi^2\right)\left(a_1^2 - \nu^2\right)\left(a_1^2 - \mu^2\right) \tag{46}$$

Now,

$$\begin{aligned} a_1^2 - \mu^2 &= a_1^2 - a_3^2 - \mu^2 + a_3^2 = \left(h_2^2 - \mu^2\right) + a_3^2 \geq a_3^2 > 0 \\ a_1^2 - \nu^2 &= a_1^2 - a_2^2 - \mu^2 + a_2^2 = \left(h_3^2 - \mu^2\right) + a_3^2 \geq a_3^2 > 0 \end{aligned} \tag{47}$$

so the condition reduces to $a_1^2 > \xi^2$.

Next, note that from the defining equation,

$$\begin{aligned} \frac{\partial \xi^2}{\partial a_1^2} &= 1 - \frac{\left(\xi^2 - a_1^2 + a_2^2\right)\left(\xi^2 - a_1^2 + a_3^2\right)\mu^2\nu^2}{\left(\mu^2 - \xi^2\right)\left(\nu^2 - \xi^2\right)\left(a_1^2 - a_2^2\right)\left(a_1^2 - a_3^2\right)} \\ \frac{\partial \xi^2}{\partial a_2^2} &= \frac{\xi^2\left(\xi^2 - a_1^2 + a_3^2\right)\left(\mu^2 - a_1^2 + a_2^2\right)\left(\nu^2 - a_1^2 + a_2^2\right)}{\left(\mu^2 - \xi^2\right)\left(\nu^2 - \xi^2\right)\left(a_1^2 - a_2^2\right)\left(a_2^2 - a_3^2\right)} \\ \frac{\partial \xi^2}{\partial a_3^2} &= -\frac{\xi^2\left(\xi^2 - a_1^2 + a_2^2\right)\left(\mu^2 - a_1^2 + a_3^2\right)\left(\nu^2 - a_1^2 + a_3^2\right)}{\left(\mu^2 - \xi^2\right)\left(\nu^2 - \xi^2\right)\left(a_1^2 - a_3^2\right)\left(a_2^2 - a_3^2\right)} \end{aligned} \tag{48}$$

so if

$$\rho\left(\mathbf{r};\mathbf{x}\right) = \rho_0 \Theta\left(a_1 - \xi\right) + \rho_1 \Theta\left(\xi - a_1\right) \tag{49}$$

then

$$\begin{aligned} \frac{\partial \rho\left(\mathbf{r};\mathbf{x}\right)}{\partial a_1} &= \left(\rho_0 - \rho_1\right)\left[\frac{-a_2^2 a_3^2}{\left(\mu^2 - a_1^2\right)\left(\nu^2 - a_1^2\right)\left(a_1^2 - a_2^2\right)\left(a_1^2 - a_3^2\right)}\right]\mu^2\nu^2\delta\left(\xi - a_1\right) + \frac{\partial \rho_1}{\partial a_1}\Theta\left(\xi - a_1\right) \\ \frac{\partial \rho\left(\mathbf{r};\mathbf{x}\right)}{\partial a_2} &= \left(\rho_0 - \rho_1\right)\left[\frac{a_1 a_2 a_3^2}{\left(\mu^2 - a_1^2\right)\left(\nu^2 - a_1^2\right)\left(a_1^2 - a_2^2\right)\left(a_2^2 - a_3^2\right)}\right]\left(\mu^2 - a_1^2 + a_2^2\right)\left(\nu^2 - a_1^2 + a_2^2\right)\delta\left(\xi - a_1\right) + \frac{\partial \rho_1}{\partial a_2}\Theta\left(\xi - a_1\right) \\ \frac{\partial \rho\left(\mathbf{r};\mathbf{x}\right)}{\partial a_3} &= \left(\rho_0 - \rho_1\right)\left[\frac{-a_1 a_2^2 a_3}{\left(\mu^2 - a_1^2\right)\left(\nu^2 - a_1^2\right)\left(a_1^2 - a_3^2\right)\left(a_2^2 - a_3^2\right)}\right]\left(\mu^2 - a_1^2 + a_3^2\right)\left(\nu^2 - a_1^2 + a_3^2\right)\delta\left(\xi - a_1\right) + \frac{\partial \rho_1}{\partial a_3}\Theta\left(\xi - a_1\right) \end{aligned} \tag{50}$$

which we can write as

$$\frac{\partial \rho\left(\mathbf{r};\mathbf{x}\right)}{\partial \mathbf{x}} = \rho\left(\mu,\nu\right)\delta\left(\xi - a_1\right) + \frac{\partial \rho_1}{\partial \mathbf{x}}\Theta\left(\xi - a_1\right) \tag{51}$$

with

$$\rho\left(\mu,\nu\right) = -\left(\rho_0 - \rho_1\right)\frac{a_1 a_2^2 a_3^2}{h_1^2 h_2^2 h_3^2}\frac{1}{\left(\mu^2 - a_1^2\right)\left(\nu^2 - a_1^2\right)}\left\{\begin{array}{c} \frac{h_1^2}{a_1}\left(\mu^2\nu^2\right) \\ \frac{h_2^2}{a_2}\left(\mu^2 - h_3^2\right)\left(h_3^2 - \nu^2\right) \\ \frac{h_3^2}{a_3}\left(h_2^2 - \mu^2\right)\left(h_2^2 - \nu^2\right) \end{array}\right\}. \tag{52}$$

### 1. *Poisson equation*

The ellipsoidal coordinates are orthogonal with scale factors

$$\begin{aligned} h_\xi &= \frac{\sqrt{\xi^2 - \mu^2}\sqrt{\xi^2 - \nu^2}}{\sqrt{\xi^2 - h_3^2}\sqrt{\xi^2 - h_2^2}} \\ h_\mu &= \frac{\sqrt{\xi^2 - \mu^2}\sqrt{\mu^2 - \nu^2}}{\sqrt{\mu^2 - h_3^2}\sqrt{h_2^2 - \mu^2}} \\ h_\nu &= \frac{\sqrt{\xi^2 - \nu^2}\sqrt{\mu^2 - \nu^2}}{\sqrt{h_3^2 - \nu^2}\sqrt{h_2^2 - \nu^2}} \end{aligned} \tag{53}$$

In these variables, we need to solve

$$\frac{1}{h_\xi(\xi,\mu,\nu)\,h_\mu(\xi,\mu,\nu)\,h_\nu(\xi,\mu,\nu)}\left\{\begin{array}{c}\frac{\partial}{\partial\xi}\rho(\xi)\,\frac{h_\mu(\xi,\mu,\nu)h_\nu(\xi,\mu,\nu)}{h_\xi(\xi,\mu,\nu)}\frac{\partial}{\partial\xi}\\ +\frac{\partial}{\partial\mu}\rho(\xi)\,\frac{h_\xi(\xi,\mu,\nu)h_\nu(\xi,\mu,\nu)}{h_\mu(\xi,\mu,\nu)}\frac{\partial}{\partial\mu}\\ +\frac{\partial}{\partial\nu}\rho(\xi)\,\frac{h_\xi(\xi,\mu,\nu)h_\mu(\xi,\mu,\nu)}{h_\nu(\xi,\mu,\nu)}\frac{\partial}{\partial\nu}\end{array}\right\}\phi(\xi,\mu,\nu)=\delta(\xi-a_1)\,\rho(\mu,\nu)+\frac{\partial\rho_1}{\partial\mathbf{x}}\Theta(\xi-a_1) \tag{54}$$

Now the differential operators can be reduced to

$$\frac{1}{h_\xi(\xi,\mu,\nu)\,h_\mu(\xi,\mu,\nu)\,h_\nu(\xi,\mu,\nu)}\frac{\partial}{\partial\xi}\frac{h_\mu(\xi,\mu,\nu)\,h_\nu(\xi,\mu,\nu)}{h_\xi(\xi,\mu,\nu)}\frac{\partial}{\partial\xi}=\frac{\sqrt{\xi^2-h_3^2}\sqrt{\xi^2-h_2^2}}{(\xi^2-\mu^2)(\xi^2-\nu^2)}\frac{\partial}{\partial\xi}\sqrt{\xi^2-h_3^2}\sqrt{\xi^2-h_2^2}\frac{\partial}{\partial\xi} \tag{55}$$

$$\frac{1}{h_\xi(\xi,\mu,\nu)\,h_\mu(\xi,\mu,\nu)\,h_\nu(\xi,\mu,\nu)}\frac{\partial}{\partial\mu}\frac{h_\xi(\xi,\mu,\nu)\,h_\nu(\xi,\mu,\nu)}{h_\mu(\xi,\mu,\nu)}\frac{\partial}{\partial\mu}=\frac{\sqrt{\mu^2-h_3^2}\sqrt{h_2^2-\mu^2}}{(\xi^2-\mu^2)(\mu^2-\nu^2)}\frac{\partial}{\partial\mu}\sqrt{\mu^2-h_3^2}\sqrt{h_2^2-\mu^2}\frac{\partial}{\partial\mu}$$

$$\frac{1}{h_\xi(\xi,\mu,\nu)\,h_\mu(\xi,\mu,\nu)\,h_\nu(\xi,\mu,\nu)}\frac{\partial}{\partial\nu}\frac{h_\xi(\xi,\mu,\nu)\,h_\mu(\xi,\mu,\nu)}{h_\nu(\xi,\mu,\nu)}\frac{\partial}{\partial\nu}=\frac{\sqrt{h_3^2-\nu^2}\sqrt{h_2^2-\nu^2}}{(\xi^2-\nu^2)(\mu^2-\nu^2)}\frac{\partial}{\partial\nu}\sqrt{h_3^2-\nu^2}\sqrt{h_2^2-\nu^2}\frac{\partial}{\partial\nu}$$

so we need to solve

$$\left\{\begin{array}{c}\frac{\sqrt{\xi^2-h_3^2}\sqrt{\xi^2-h_2^2}}{(\xi^2-\mu^2)(\xi^2-\nu^2)}\frac{\partial}{\partial\xi}\rho(\xi)\,\sqrt{\xi^2-h_3^2}\sqrt{\xi^2-h_2^2}\frac{\partial}{\partial\xi}\\ +\rho(\xi)\,\frac{\sqrt{\mu^2-h_3^2}\sqrt{h_2^2-\mu^2}}{(\xi^2-\mu^2)(\mu^2-\nu^2)}\frac{\partial}{\partial\mu}\sqrt{\mu^2-h_3^2}\sqrt{h_2^2-\mu^2}\frac{\partial}{\partial\mu}\\ +\rho(\xi)\,\frac{\sqrt{h_3^2-\nu^2}\sqrt{h_2^2-\nu^2}}{(\xi^2-\nu^2)(\mu^2-\nu^2)}\frac{\partial}{\partial\nu}\sqrt{h_3^2-\nu^2}\sqrt{h_2^2-\nu^2}\frac{\partial}{\partial\nu}\end{array}\right\}\phi(\xi,\mu,\nu)=\delta(\xi-a_1)\,\rho(\mu,\nu)+\frac{\partial\rho_1}{\partial\mathbf{x}}\Theta(\xi-a_1) \tag{56}$$

### *2. Separation into different regions*

We guess that the solution can be written as

$$\phi(\xi,\mu,\nu)=\phi_0(\xi,\mu,\nu)\,\Theta(a_1-\xi)+\phi_1(\xi,\mu,\nu)\,\Theta(\xi-a_1) \tag{57}$$

Then we have only to treat the different delta functions that arise. Note that, e.g.,

$$\begin{aligned}&\frac{\partial}{\partial\xi}\rho(\xi)\,\sqrt{\xi^2-h_3^2}\sqrt{\xi^2-h_2^2}\frac{\partial}{\partial\xi}\phi_0(\xi,\mu,\nu)\,\Theta(a_1-\xi)\\ &=-\frac{\partial}{\partial\xi}\rho(\xi)\,\sqrt{\xi^2-h_3^2}\sqrt{\xi^2-h_2^2}\phi_0(\xi,\mu,\nu)\,\delta(a_1-\xi)\\ &+\frac{\partial}{\partial\xi}\rho(\xi)\,\sqrt{\xi^2-h_3^2}\sqrt{\xi^2-h_2^2}\Theta(a_1-\xi)\,\frac{\partial}{\partial\xi}\phi_0(\xi,\mu,\nu)\end{aligned} \tag{58}$$

and the right hand side can be written as

$$\begin{aligned}&-\rho(a_1)\,a_2a_3\phi_0(a_1,\mu,\nu)\,\frac{\partial}{\partial\xi}\delta(a_1-\xi)\\ &+\rho_0\frac{\partial}{\partial\xi}\sqrt{\xi^2-h_3^2}\sqrt{\xi^2-h_2^2}\Theta(a_1-\xi)\,\frac{\partial}{\partial\xi}\phi_0(\xi,\mu,\nu)\end{aligned} \tag{59}$$

and

$$\begin{aligned}&-\rho(a_1)\,a_2a_3\phi_0(a_1,\mu,\nu)\,\frac{\partial}{\partial\xi}\delta(a_1-\xi)\\ &-\left(\rho_0a_2a_3\frac{\partial}{\partial\xi}\phi_0(\xi,\mu,\nu)\right)\delta(a_1-\xi)\\ &+\rho_0\Theta(a_1-\xi)\,\frac{\partial}{\partial\xi}\sqrt{\xi^2-h_3^2}\sqrt{\xi^2-h_2^2}\frac{\partial}{\partial\xi}\phi_0(\xi,\mu,\nu)\end{aligned} \tag{60}$$

So we have that

$$\delta(\xi-a_1)\rho(\mu,\nu)+\frac{\partial\rho_1}{\partial\mathbf{x}}\Theta(\xi-a_1)=\frac{\sqrt{\xi^2-h_3^2}\sqrt{\xi^2-h_2^2}}{(\xi^2-\mu^2)(\xi^2-\nu^2)}\rho(a_1)a_2a_3(\phi_1(a_1,\mu,\nu)-\phi_0(a_1,\mu,\nu))\frac{\partial}{\partial\xi}\delta(\xi-a_1) \tag{61}$$
$$+\frac{a_2^2a_3^2}{(a_1^2-\mu^2)(a_1^2-\nu^2)}\left(\rho_1\left(\frac{\partial\phi_1(\xi,\mu,\nu)}{\partial\xi}\right)_{a_1}-\rho_0\left(\frac{\partial\phi_0(\xi,\mu,\nu)}{\partial\xi}\right)_{a_1}\right)\delta(a_1-\xi)$$
$$+\Theta(a_1-\xi)\rho_0\nabla^2\phi_0(\xi,\mu,\nu)+\Theta(\xi-a_1)\rho_1\nabla^2\phi_1(\xi,\mu,\nu)$$

from which we find that

$$\phi_1(a_1,\mu,\nu)=\phi_0(a_1,\mu,\nu) \tag{62}$$
$$\frac{(a_1^2-\mu^2)(a_1^2-\nu^2)}{a_2^2a_3^2}\rho(\mu,\nu)=\rho_1\left(\frac{\partial\phi_1(\xi,\mu,\nu)}{\partial\xi}\right)_{a_1}-\rho_0\left(\frac{\partial\phi_0(\xi,\mu,\nu)}{\partial\xi}\right)_{a_1}$$
$$\Theta(a_1-\xi)\nabla^2\phi_0(\xi,\mu,\nu)=0$$
$$\Theta(\xi-a_1)\nabla^2\phi_1(\xi,\mu,\nu)=\Theta(\xi-a_1)\frac{1}{\rho_1}\frac{\partial\rho_1}{\partial\mathbf{x}}$$

### *3. Solution*

It turns out that Laplace's equation is separable in ellipsoidal coordinates (which is why they are used). The general solution has the form

$$\phi_0^{(\alpha)}(\mathbf{r})=\sum_{n=0}^{\infty}\sum_{p=1}^{2n+1}\left(A_{np}^{(\alpha)}E_n^p(\xi)+B_{np}^{(\alpha)}F_n^p(\xi)\right)E_n^p(\mu)E_n^p(\nu) \tag{63}$$
$$\phi_1^{(\alpha)}(\mathbf{r})=\sum_{n=0}^{\infty}\sum_{p=1}^{2n+1}\left(A_{np}^{\prime(\alpha)}E_n^p(\xi)+B_{np}^{\prime(\alpha)}F_n^p(\xi)\right)E_n^p(\mu)E_n^p(\nu)$$

where the parameter $\alpha$ refers to the order-parameter. Here, $E_n^p(x)$ are the Lame functions of the first kind (polynomials and more complex algebraic functions) and the Lame functions of the second kind are $F_n^p(\xi)$ (which generally take the form of incomplete elliptic integrals). The combinations $E_n^p(\xi)E_n^p(\mu)E_n^p(\nu)$ are called the inner ellipsoidal harmonics and the combination $F_n^p(\xi)E_n^p(\mu)E_n^p(\nu)$the outer ellipsoidal harmonics. The parts in $\mu$ and $\nu$ are called the surface harmonics and are analagous to spherical harmonics. On the other hand, $E_n^p(\xi)$ is regular for $\xi\to h_2$ (the minimum allowed value of this coordinate - see above) and $F_n^p(\xi)$ behaves as $\xi^{-n-1}$for $\xi\gg 1$. So this combination of inner and outer harmonics is chosen to be regular in the interior of the cluster and to not blow up as $\xi$ becomes large.

To simplify the notation, I treat the combination of $np$ as a single index and so that $A_{np}^{(\alpha)},B_{np}^{(\alpha)}$ etc can be viewed as matrices of size $N\times M$ where $N$ is the number of parameters in the density and $M$ is the number of ellipsoidal harmonics that we keep in the sums in Eq.(63) (which in principle is inifinite but which we will find reduces to only 3 for our problem). These matrices will be denoted in bold as $\mathbf{A},\mathbf{B}$ etc. next, we define $\mathcal{E}(\xi)$ and $\mathcal{F}(\xi)$ as the $M\times M$ diagonal matrices with $E_n^p(\xi)$ and $F_n^p(\xi)$ on the diagonals and $\ominus(\mu,\nu)$ as the $M\times 1$ vector with elements $E_n^p(\mu)E_n^p(\nu)$. Then we can write Eq(63) as

$$\phi_0(\mathbf{r})=(\mathbf{A}\mathcal{E}(\xi)+\mathbf{B}\mathcal{F}(\xi))\ominus(\mu,\nu) \tag{64}$$
$$\phi_1(\mathbf{r})=(\mathbf{A}'\mathcal{E}(\xi)+\mathbf{B}'\mathcal{F}(\xi))\ominus(\mu,\nu)$$

The general solution to our problem (which has a source term on the right hand) will be the sum of this general homogeneous solution and a particular solution which is denoted as $\overline{\phi}(\mathbf{r})$ so that we can write

$$\phi_0(\mathbf{r})=(\mathbf{A}\mathcal{E}(\xi)+\mathbf{B}\mathcal{F}(\xi))\ominus(\mu,\nu)+\mathbf{C}(\xi)\ominus(\mu,\nu) \tag{65}$$
$$\phi_1(\mathbf{r})=(\mathbf{A}'\mathcal{E}(\xi)+\mathbf{B}'\mathcal{F}(\xi))\ominus(\mu,\nu)+\mathbf{C}'(\xi)\ominus(\mu,\nu)$$

where it is to be noted that $\mathbf{C}(\xi)$ does not necessarily have the form $\overline{\mathbf{A}}\mathcal{E}(\xi)$. In order to make the following more compact, I will also write $\mathbf{A}\mathcal{E}(\xi)$ as $\mathbf{A}(\xi)$, etc.

The derivatives of the density at the discontinuity can be written in terms of the Lame functions (see Appendix A) as

$$\frac{\left(a_1^2-\mu^2\right)\left(a_1^2-\nu^2\right)}{a_2^2 a_3^2}\rho\left(\mu,\nu\right)=-\left(\rho_0-\rho_1\right)a_1\mathbf{U}\ominus\left(\mu,\nu\right) \tag{66}$$

where $\mathbf{U}$ is again an $N\times M$ matrix. Explicitly,

$$\mathbf{U}=\begin{pmatrix} \frac{1}{3a_1} & -\frac{1}{a_1h_2^2h_3^2}\frac{\Lambda_2-a_1^2}{\Lambda_1-\Lambda_2} & \frac{1}{a_1h_2^2h_3^2}\frac{\Lambda_1-a_1^2}{\Lambda_1-\Lambda_2} \\ \frac{1}{3a_2} & \frac{1}{a_2h_1^2h_3^2}\frac{\Lambda_2-a_2^2}{\Lambda_1-\Lambda_2} & -\frac{1}{a_2h_1^2h_3^2}\frac{\Lambda_1-a_2^2}{\Lambda_1-\Lambda_2} \\ \frac{1}{3a_3} & -\frac{1}{a_3h_1^2h_2^2}\frac{\Lambda_2-a_3^2}{\Lambda_1-\Lambda_2} & \frac{1}{a_3h_1^2h_2^2}\frac{\Lambda_1-a_3^2}{\Lambda_1-\Lambda_2} \end{pmatrix} \tag{67}$$

with

$$\begin{aligned}\Lambda_1&=\frac{1}{3}\left(a_1^2+a_2^2+a_3^2+\sqrt{a_1^4+a_2^4+a_3^4-a_1^2a_2^2-a_1^2a_3^2-a_2^2a_3^2}\right)\\ \Lambda_2&=\frac{1}{3}\left(a_1^2+a_2^2+a_3^2-\sqrt{a_1^4+a_2^4+a_3^4-a_1^2a_2^2-a_1^2a_3^2-a_2^2a_3^2}\right)\end{aligned} \tag{68}$$

where we note that it only has nonzero entries for $(np)=(01),(2,1)$ and $(2,2)$ so all other entries are suppressed. It turns out that the particular solution also is restricted to this subspace so that from now on, we can restrict all sums, matrices and vectors to this subspace. This means, e.g., that $\mathbf{A},\mathbf{B}$ etc are of size $3\times 3$, $\ominus$ is $3\times 1$ etc. Finally, the conditions that must be obeyed at the discontinuity take the form

$$\left(\mathbf{A}\left(a_1\right)+\mathbf{B}\left(a_1\right)+\mathbf{C}\left(a_1\right)\right)\ominus\left(\mu,\nu\right)=\left(\mathbf{A}'\left(a_1\right)+\mathbf{B}'\left(a_1\right)+\mathbf{C}'\left(a_1\right)\right)\ominus\left(\mu,\nu\right) \tag{69}$$

and

$$\begin{aligned}&\left(\rho_\infty\left(\frac{d}{d\xi}\mathbf{A}'\left(\xi\right)+\frac{d}{d\xi}\mathbf{B}'\left(\xi\right)+\frac{d}{d\xi}\mathbf{C}'\left(\xi\right)\right)-\rho_0\left(\frac{d}{d\xi}\mathbf{A}\left(\xi\right)+\frac{d}{d\xi}\mathbf{B}\left(\xi\right)+\frac{d}{d\xi}\mathbf{C}\left(\xi\right)\right)\right)_{\xi=a_1}\ominus\left(\mu,\nu\right)\\ &\qquad=-\left(\rho_0-\rho_1\right)a_1\mathbf{U}\ominus\left(\mu,\nu\right)\end{aligned}$$

The orthogonality condition

$$\int_0^h d\nu\int_h^k d\mu\frac{\mu^2-\nu^2}{\sqrt{\left(\mu^2-h^2\right)\left(k^2-\mu^2\right)\left(h^2-\nu^2\right)\left(k^2-\nu^2\right)}}\ominus\left(\mu,\nu\right)\ominus\left(\mu,\nu\right)=\gamma, \tag{70}$$

where $\gamma$ is a (known) diagonal matrix of constants, allows us to reduce these to

$$\mathbf{A}\left(a_1\right)+\mathbf{B}\left(a_1\right)+\mathbf{C}\left(a_1\right)=\mathbf{A}'\left(a_1\right)+\mathbf{B}'\left(a_1\right)+\mathbf{C}'\left(a_1\right) \tag{71}$$

and

$$\begin{aligned}&\rho_\infty\left(\frac{d}{d\xi}\mathbf{A}'\left(\xi\right)\right)_{\xi=a_1}+\rho_\infty\left(\frac{d}{d\xi}\mathbf{B}'\left(\xi\right)\right)_{\xi=a_1}+\rho_\infty\left(\frac{d}{d\xi}\mathbf{C}'\left(\xi\right)\right)_{\xi=a_1}\\ &\qquad-\rho_0\left(\frac{d}{d\xi}\mathbf{A}\left(\xi\right)\right)_{\xi=a_1}-\rho_0\left(\frac{d}{d\xi}\mathbf{B}\left(\xi\right)\right)_{\xi=a_1}-\rho_0\left(\frac{d}{d\xi}\mathbf{C}\left(\xi\right)\right)_{\xi=a_1}\\ &\qquad=-\left(\rho_0-\rho_1\right)a_1\mathbf{U}\end{aligned}$$

Hence, we have that

$$\mathbf{A}=-\mathbf{B}\left(a_1\right)\mathcal{E}^{-1}\left(a_1\right)-\mathbf{C}\left(a_1\right)\mathcal{E}^{-1}\left(a_1\right)+\mathbf{A}'+\mathbf{B}'\left(a_1\right)\mathcal{E}^{-1}\left(a_1\right)+\mathbf{C}'\left(a_1\right)\mathcal{E}^{-1}\left(a_1\right) \tag{72}$$

and

$$(\rho_\infty - \rho_0)\left(\frac{d}{d\xi}\mathbf{A}'(\xi)\right)_{\xi=a_1} + \mathbf{B}'\left[\rho_\infty\left(\frac{d}{d\xi}\mathcal{F}(\xi)\right)_{\xi=a_1} - \rho_0\mathcal{F}(a_1)\mathcal{E}^{-1}(a_1)\left(\frac{d}{d\xi}\mathcal{E}(\xi)\right)_{\xi=a_1}\right]$$
$$+\rho_0\mathbf{B}\left[\mathcal{F}(a_1)\mathcal{E}^{-1}(a_1)\left(\frac{d}{d\xi}\mathcal{E}(\xi)\right)_{\xi=a_1} - \left(\frac{d}{d\xi}\mathcal{F}(\xi)\right)_{\xi=a_1}\right]$$
$$+\rho_0\mathbf{C}(a_1)\mathcal{E}^{-1}(a_1)\left(\frac{d}{d\xi}\mathcal{E}(\xi)\right)_{\xi=a_1} - \rho_0\left(\frac{d}{d\xi}\mathbf{C}(\xi)\right)_{\xi=a_1}$$
$$+\rho_\infty\left(\frac{d}{d\xi}\mathbf{C}'(\xi)\right)_{\xi=a_1} - \rho_0\mathbf{C}'(a_1)\mathcal{E}^{-1}(a_1)\left(\frac{d}{d\xi}\mathcal{E}(\xi)\right)_{\xi=a_1}$$
$$= -(\rho_0-\rho_1)a_1\mathbf{U}$$

Using the Wronskian,

$$\mathcal{E}(\xi)\frac{d}{d\xi}\mathcal{F}(\xi) - \left(\frac{d}{d\xi}\mathcal{E}(\xi)\right)\mathcal{F}(\xi) = -\frac{1}{\sqrt{\xi^2-h_2^2}\sqrt{\xi^2-h_3^2}}\mathcal{W} \tag{73}$$

with $\mathcal{W}_{np,n'p'} = \delta_{nn'}\delta_{pp'}(2n+1)$, gives

$$\left(\frac{d}{d\xi}\mathcal{F}(\xi)\right)_{a_1} = \mathcal{E}^{-1}(a_1)\left(\frac{d}{d\xi}\mathcal{E}(\xi)\right)_{a_1}\mathcal{F}(a_1) - \frac{1}{a_2a_3}\mathcal{E}^{-1}(a_1)\mathcal{W} \tag{74}$$

and

$$(\rho_1-\rho_0)\left(\frac{d}{d\xi}\mathbf{A}'(\xi)\right)_{\xi=a_1} - \mathbf{B}'\frac{1}{a_2a_3}\mathcal{E}^{-1}(a_1)\left[a_2a_3(\rho_0-\rho_\infty)\left(\frac{d}{d\xi}\mathcal{E}(\xi)\right)\mathcal{F}(a_1)+\rho_1\mathcal{W}\right] \tag{75}$$
$$+\frac{\rho_0}{a_2a_3}\mathbf{B}\mathcal{E}^{-1}(a_1)\mathcal{W}$$
$$+\rho_0\mathbf{C}(a_1)\mathcal{E}^{-1}(a_1)\left(\frac{d}{d\xi}\mathcal{E}(\xi)\right)_{\xi=a_1} - \rho_0\left(\frac{d}{d\xi}\mathbf{C}(\xi)\right)_{\xi=a_1}$$
$$+\rho_1\left(\frac{d}{d\xi}\mathbf{C}'(\xi)\right)_{\xi=a_1} - \rho_0\mathbf{C}'(a_1)\mathcal{E}^{-1}(a_1)\left(\frac{d}{d\xi}\mathcal{E}(\xi)\right)_{\xi=a_1}$$
$$= -(\rho_0-\rho_1)a_1\mathbf{U}$$

or

$$\mathbf{B}' = (\rho_0-\rho_1)(a_1a_2a_3)\mathbf{U}\mathcal{E}(a_1)\left[a_2a_3(\rho_0-\rho_1)\left(\frac{d}{d\xi}\mathcal{E}(\xi)\right)\mathcal{F}(a_1)+\rho_\infty\mathcal{W}\right]^{-1} \tag{76}$$
$$+\left((\rho_1-\rho_0)a_2a_3\mathbf{A}'\left(\frac{d}{d\xi}\mathcal{E}(\xi)\right)_{\xi=a_1}\mathcal{E}(a_1)+\rho_0\mathbf{B}\mathcal{W}\right)\left[a_2a_3(\rho_0-\rho_1)\left(\frac{d}{d\xi}\mathcal{E}(\xi)\right)\mathcal{F}(a_1)+\rho_1\mathcal{W}\right]^{-1}$$
$$+\rho_0a_2a_3\left(\mathbf{C}(a_1)\left(\frac{d}{d\xi}\mathcal{E}(\xi)\right)_{\xi=a_1} - \left(\frac{d}{d\xi}\mathbf{C}(\xi)\right)_{\xi=a_1}\mathcal{E}(a_1)\right)\left[a_2a_3(\rho_0-\rho_1)\left(\frac{d}{d\xi}\mathcal{E}(\xi)\right)\mathcal{F}(a_1)+\rho_1\mathcal{W}\right]^{-1}$$
$$+a_2a_3\left(\rho_\infty\left(\frac{d}{d\xi}\mathbf{C}'(\xi)\right)_{\xi=a_1}\mathcal{E}(a_1) - \rho_0\mathbf{C}'(a_1)\left(\frac{d}{d\xi}\mathcal{E}(\xi)\right)_{\xi=a_1}\right)\left[a_2a_3(\rho_0-\rho_1)\left(\frac{d}{d\xi}\mathcal{E}(\xi)\right)\mathcal{F}(a_1)+\rho_1\mathcal{W}\right]^{-1}$$

If we use the natural boundary conditions, then we take $\mathbf{A}'=\mathbf{B}=\mathbf{0}$ and

$$\mathbf{B}' = (\rho_0-\rho_1)(a_1a_2a_3)\mathbf{U}\mathcal{E}(a_1)\left[a_2a_3(\rho_0-\rho_1)\left(\frac{d}{d\xi}\mathcal{E}(\xi)\right)\mathcal{F}(a_1)+\rho_{1\infty}\mathcal{W}\right]^{-1} \tag{77}$$
$$+\rho_0a_2a_3\left(\mathbf{C}(a_1)\left(\frac{d}{d\xi}\mathcal{E}(\xi)\right)_{\xi=a_1} - \left(\frac{d}{d\xi}\mathbf{C}(\xi)\right)_{\xi=a_1}\mathcal{E}(a_1)\right)\left[a_2a_3(\rho_0-\rho_1)\left(\frac{d}{d\xi}\mathcal{E}(\xi)\right)\mathcal{F}(a_1)+\rho_\infty\mathcal{W}\right]^{-1}$$
$$+a_2a_3\left(\rho_1\left(\frac{d}{d\xi}\mathbf{C}'(\xi)\right)_{\xi=a_1}\mathcal{E}(a_1) - \rho_0\mathbf{C}'(a_1)\left(\frac{d}{d\xi}\mathcal{E}(\xi)\right)_{\xi=a_1}\right)\left[a_2a_3(\rho_0-\rho_1)\left(\frac{d}{d\xi}\mathcal{E}(\xi)\right)\mathcal{F}(a_1)+\rho_\infty\mathcal{W}\right]^{-1}$$

In general, the terms $\mathbf{C}$ and $\mathbf{C}'$ will scale as the inverse of the total radius and so are negligable in the large system limit leaving

$$\mathbf{B}' = (\rho_0 - \rho_1)(a_1 a_2 a_3)\,\mathbf{U}\mathcal{E}(a_1)\left[a_2 a_3 (\rho_0 - \rho_1)\left(\frac{d}{d\xi}\mathcal{E}(\xi)\right)\mathcal{F}(a_1) + \rho_1 \mathcal{W}\right]^{-1} \tag{78}$$

Explicitly,

$$[] = \begin{pmatrix} \rho_1 & 0 & 0 \\ 0 & 2a_1a_2a_3(\rho_0-\rho_1)F_{12}(a_1)+5\rho_1 & 0 \\ 0 & 0 & 2a_1a_2a_3(\rho_0-\rho_1)F_{22}(a_1)+5\rho_1 \end{pmatrix} \tag{79}$$

and we will need

$$(\phi(\mathbf{r}))_{\xi=a_1} = \{\mathbf{A}'\mathcal{E}(a_1) + \mathbf{B}'\mathcal{F}(a_1) + \mathbf{C}'(a_1)\}\ominus(\mu,\nu)$$

## B. Metric

We now need

$$\begin{aligned} \mathbf{g} &= -\int \frac{\partial\rho(\mathbf{r})}{\partial\mathbf{x}}\phi(\mathbf{r})\,d\mathbf{r} \\ &= -\int_{h_2}^{\infty} d\xi \int_{h_3}^{h_2} d\mu \int_0^{h_3} d\nu\, h_\xi(\xi,\mu,\nu)\, h_\mu(\xi,\mu,\nu)\, h_\nu(\xi,\mu,\nu)\,\frac{\partial\rho(\mathbf{r})}{\partial\mathbf{X}}\phi(\mathbf{r}) \\ &= -\int_{h_2}^{\infty} d\xi \int_{h_3}^{h_2} d\mu \int_0^{h_3} d\nu \frac{(\xi^2-\mu^2)(\xi^2-\nu^2)(\mu^2-\nu^2)}{\sqrt{\xi^2-h_3^2}\sqrt{\xi^2-h_2^2}\sqrt{\mu^2-h_3^2}\sqrt{h_2^2-\mu^2}\sqrt{h_3^2-\nu^2}\sqrt{h_2^2-\nu^2}}\frac{\partial\rho(\mathbf{r})}{\partial\mathbf{X}}\phi(\mathbf{r}) \end{aligned} \tag{80}$$

Substituting

$$\frac{\partial\rho(\mathbf{r})}{\partial\mathbf{x}} = \delta(\xi - a_1)\,\rho(\mu,\nu) + \frac{\partial\rho_1}{\partial\mathbf{x}}\Theta(\xi - a_1) \tag{81}$$

gives

$$\begin{aligned} \mathbf{g} = &-\frac{1}{a_2a_3}\int_{h_3}^{h_2} d\mu \int_0^{h_3} d\nu \frac{(a_1^2-\mu^2)(a_1^2-\nu^2)(\mu^2-\nu^2)}{\sqrt{\mu^2-h_3^2}\sqrt{h_2^2-\mu^2}\sqrt{h_3^2-\nu^2}\sqrt{h_2^2-\nu^2}}\rho(\mu,\nu)\,\phi(\mathbf{r}) \\ &-\frac{\partial\rho_1}{\partial\mathbf{x}}\int_{a_1}^{\infty} d\xi \int_{h_3}^{h_2} d\mu \int_0^{h_3} d\nu \frac{(\xi^2-\mu^2)(\xi^2-\nu^2)(\mu^2-\nu^2)}{\sqrt{\xi^2-h_3^2}\sqrt{\xi^2-h_2^2}\sqrt{\mu^2-h_3^2}\sqrt{h_2^2-\mu^2}\sqrt{h_3^2-\nu^2}\sqrt{h_2^2-\nu^2}}\phi(\mathbf{r})\,. \end{aligned} \tag{82}$$

### 1. *First contribution*

From Eq.(66) we get

$$\mathbf{g}_1 = (\rho_0 - \rho_1)\,a_1a_2a_3 \int_{h_3}^{h_2} d\mu \int_0^{h_3} d\nu \frac{(\mu^2-\nu^2)}{\sqrt{\mu^2-h_3^2}\sqrt{h_2^2-\mu^2}\sqrt{h_3^2-\nu^2}\sqrt{h_2^2-\nu^2}}\mathbf{U}\ominus(\mu,\nu)\,\phi(\mathbf{r}) \tag{83}$$

and substituting for the potential

$$\begin{aligned} \mathbf{g}_1 &= (\rho_0 - \rho_1)\,a_1a_2a_3 \int_{h_3}^{h_2} d\mu \int_0^{h_3} d\nu \frac{(\mu^2-\nu^2)}{\sqrt{\mu^2-h_3^2}\sqrt{h_2^2-\mu^2}\sqrt{h_3^2-\nu^2}\sqrt{h_2^2-\nu^2}} \\ &\quad\times \mathbf{U}\ominus(\mu,\nu)\ominus^T(\mu,\nu)\left\{\mathcal{E}(a_1)\,\mathbf{A}'^T + \mathcal{F}(a_1)\,\mathbf{B}'^T + \mathbf{C}'^T(a_1)\right\} \\ &= (\rho_0-\rho_1)\,a_2a_3\mathbf{U}\gamma\left\{\mathcal{E}(a_1)\,\mathbf{A}'^T + \mathcal{F}(a_1)\,\mathbf{B}'^T + \mathbf{C}'^T(a_1)\right\} \end{aligned} \tag{84}$$

using the orthogonality relation. This is the general result and we can substitute the expression for $\mathbf{B}'^T$ to get an explicit expression. If we assume the natural boundary conditions and take the large system limit, we get

$$\begin{aligned}\mathbf{g}_1 &= (\rho_0-\rho_1)\, a_1a_2a_3\mathbf{U}\gamma\mathcal{F}(a_1)\,\mathbf{B}'^T \\ &= (\rho_0-\rho_1)^2 (a_1a_2a_3)^2\,\mathbf{U}\gamma\mathcal{F}(a_1)\left[a_2a_3(\rho_0-\rho_1)\left(\frac{d}{d\xi}\mathcal{E}(\xi)\right)_{a_1}\mathcal{F}(a_1)+\rho_1\mathcal{W}\right]^{-1}\mathcal{E}(a_1)\,\mathbf{U}^T \\ &= \gamma_{01}(\rho_0-\rho_1)^2(a_1a_2a_3)^2\,\mathbf{U}\mathbf{D}\mathbf{U}^T\end{aligned} \tag{85}$$

with

$$\begin{aligned}\mathbf{D}_{11} &= \frac{F_{01}(a_1)}{\rho_1} \\ \mathbf{D}_{22} &= \frac{F_{21}(a_1)}{2a_1a_2a_3(\rho_0-\rho_1)F_{21}(a_1)+5\rho_1}\frac{\gamma_{21}}{\gamma_{01}}\Lambda_1 \\ \mathbf{D}_{33} &= \frac{F_{22}(a_1)}{2a_1a_2a_3(\rho_0-\rho_1)F_{22}(a_1)+5\rho_1}\frac{\gamma_{22}}{\gamma_{01}}\Lambda_2\end{aligned} \tag{86}$$

In particular, we can calculate

$$\begin{aligned}\det\mathbf{g}_1 &= \left((\rho_0-\rho_1)^2(a_1a_2a_3)^2\right)^3(\det\mathbf{U})^2\,\gamma_{01}\gamma_{21}\gamma_{22} \\ &\times\frac{F_{01}(a_1)}{\rho_1}\frac{F_{21}(a_1)}{2a_1a_2a_3(\rho_0-\rho_1)F_{21}(a_1)+5\rho_1}\frac{F_{22}(a_1)}{2a_1a_2a_3(\rho_0-\rho_1)F_{22}(a_1)+5\rho_1}\Lambda_1\Lambda_2\end{aligned} \tag{87}$$

A short calculation gives

$$(\det\mathbf{U})^2\,\gamma_{01}\gamma_{21}\gamma_{22}\Lambda_1\Lambda_2 = \frac{256}{2025}\frac{\pi^3}{a_1^2a_2^2a_3^2}\left(a_1^2a_2^2+a_1^2a_3^2+a_2^2a_3^2\right) \tag{88}$$

so

$$\begin{aligned}\det\mathbf{g}_1 &= \frac{256}{2025}\pi^3\frac{(\rho_0-\rho_1)^6}{\rho_1}(a_1a_2a_3)^4\left(a_1^2a_2^2+a_1^2a_3^2+a_2^2a_3^2\right) \\ &\times F_{01}(a_1)\frac{F_{21}(a_1)}{2a_1a_2a_3(\rho_0-\rho_1)F_{21}(a_1)+5\rho_1}\frac{F_{22}(a_1)}{2a_1a_2a_3(\rho_0-\rho_1)F_{22}(a_1)+5\rho_1}\end{aligned} \tag{89}$$

In the weak solution limit this becomes

$$\det\mathbf{g}_1 = \frac{64}{2025}\pi^3\frac{\rho_0^4}{\rho_1}(a_1a_2a_3)^2\left(a_1^2a_2^2+a_1^2a_3^2+a_2^2a_3^2\right)F_{01}(a_1)\,. \tag{90}$$

### C. Physical Coordinates

It is interesting to separate the size and shape degrees of freedom by introducing a kind of radius and the eccentricities as the variables. Thus, define

$$\begin{aligned}R &= (a_1a_2a_3)^{1/3} \\ \varepsilon_1 &= \sqrt{\frac{a_1^2-a_2^2}{a_1^2}} \\ \varepsilon_2 &= \sqrt{\frac{a_1^2-a_3^2}{a_1^2}}\end{aligned} \tag{91}$$

giving

$$
\begin{aligned}
a_1 &= \frac{R}{\left(1-\varepsilon_1^2\right)^{1/6}\left(1-\varepsilon_2^2\right)^{1/6}} \\
a_2 &= \frac{R}{\left(1-\varepsilon_1^2\right)^{1/6}\left(1-\varepsilon_2^2\right)^{1/6}}\left(1-\varepsilon_1^2\right)^{1/2} \\
a_3 &= \frac{R}{\left(1-\varepsilon_1^2\right)^{1/6}\left(1-\varepsilon_2^2\right)^{1/6}}\left(1-\varepsilon_2^2\right)^{1/2}
\end{aligned} \tag{92}
$$

and

$$
\begin{aligned}
h_1^2 &= a_1^2\left(\varepsilon_2^2-\varepsilon_1^2\right) \\
h_2^2 &= a_1^2\varepsilon_2^2 \\
h_3^2 &= a_1^2\varepsilon_1^2
\end{aligned} \tag{93}
$$

The transformation law for the metric is

$$
\overline{g}_{ab} = \frac{\partial X^i}{\partial Y^a} g_{ij} \frac{\partial X^j}{\partial Y^b}
$$

Now, the transformed matrix is $\mathbf{VU}$ with

$$
\mathbf{V}_a^i = \frac{\partial X^i}{\partial Y^a} = \begin{pmatrix}
\frac{1}{3}\left(1-\varepsilon_1^2\right)^{1/6}\left(1-\varepsilon_2^2\right)^{1/6} & \frac{1}{3}\frac{\left(1-\varepsilon_1^2\right)^{1/6}\left(1-\varepsilon_2^2\right)^{1/6}}{\left(1-\varepsilon_1^2\right)^{1/2}} & \frac{1}{3}\frac{\left(1-\varepsilon_1^2\right)^{1/6}\left(1-\varepsilon_2^2\right)^{1/6}}{\left(1-\varepsilon_2^2\right)^{1/2}} \\
-\frac{1}{\varepsilon_1}\left(\varepsilon_1^2-1\right) & -\frac{1}{R\varepsilon_1}\left(1-\varepsilon_1^2\right)^{\frac{2}{3}}\sqrt[6]{1-\varepsilon_2^2} & 0 \\
\frac{1}{R\varepsilon_2}\sqrt[6]{1-\varepsilon_1^2}\left(1-\varepsilon_2^2\right)^{\frac{7}{6}} & 0 & -\frac{1}{R\varepsilon_2}\sqrt[6]{1-\varepsilon_1^2}\left(1-\varepsilon_2^2\right)^{\frac{2}{3}}
\end{pmatrix} \tag{94}
$$

and eventually

$$
\begin{aligned}
&\left(\overline{\mathbf{g}}_1\right)_{11} = \left(\rho_0-\rho_1\right)^2 R^4 d_0 \\
&\left(\overline{\mathbf{g}}_1\right)_{12} = \left(\overline{\mathbf{g}}_1\right)_{13} = \left(\overline{\mathbf{g}}_1\right)_{21} = \left(\overline{\mathbf{g}}_1\right)_{31} = 0 \\
&\left(\overline{\mathbf{g}}_1\right)_{22} = \left(\rho_0-\rho_1\right)^2 \frac{1}{4R^2}\frac{\left(1-\varepsilon_2^2\right)^{\frac{4}{3}}}{\varepsilon_1^2\left(1-\varepsilon_1^2\right)^{\frac{2}{3}}\left(\varepsilon_1^2-\varepsilon_2^2\right)^2\left(\varepsilon_1^4-\varepsilon_1^2\varepsilon_2^2+\varepsilon_2^4\right)}\begin{pmatrix}\left(5\varepsilon_1^4+2\varepsilon_2^4-5\varepsilon_1^2\varepsilon_2^2\right)\left(d_1+d_2\right) \\ -2\left(2\varepsilon_1^2-\varepsilon_2^2\right)\left(d_1-d_2\right)\sqrt{\varepsilon_1^4+\varepsilon_2^4-\varepsilon_1^2\varepsilon_2^2}\end{pmatrix} \\
&\left(\overline{\mathbf{g}}_1\right)_{23} = \left(\overline{\mathbf{g}}_1\right)_{32} = \left(\rho_0-\rho_1\right)^2 \frac{1}{4R^2}\frac{\sqrt[3]{1-\varepsilon_1^2}\sqrt[3]{1-\varepsilon_2^2}}{\varepsilon_1\varepsilon_2\left(\varepsilon_1^2-\varepsilon_2^2\right)^2\left(\varepsilon_1^4-\varepsilon_1^2\varepsilon_2^2+\varepsilon_2^4\right)}\begin{pmatrix}\left(\varepsilon_1^4+\varepsilon_2^4-4\varepsilon_1^2\varepsilon_2^2\right)\left(d_1+d_2\right) \\ +\left(\varepsilon_1^2+\varepsilon_2^2\right)\sqrt{\varepsilon_1^4+\varepsilon_2^4-\varepsilon_1^2\varepsilon_2^2}\left(d_1-d_2\right)\end{pmatrix} \\
&\left(\overline{\mathbf{g}}_1\right)_{33} = \left(\rho_0-\rho_1\right)^2 \frac{1}{4R^2\varepsilon_2^2}\frac{\left(1-\varepsilon_1^2\right)^{\frac{4}{3}}}{\left(1-\varepsilon_2^2\right)^{\frac{2}{3}}\left(\varepsilon_1^2-\varepsilon_2^2\right)^2\left(\varepsilon_1^4-\varepsilon_1^2\varepsilon_2^2+\varepsilon_2^4\right)}\begin{pmatrix}\left(2\varepsilon_1^4+5\varepsilon_2^4-5\varepsilon_1^2\varepsilon_2^2\right)\left(d_1+d_2\right) \\ +2\sqrt{\varepsilon_1^4+\varepsilon_2^4-\varepsilon_1^2\varepsilon_2^2}\left(\varepsilon_1^2-2\varepsilon_2^2\right)\left(d_1-d_2\right)\end{pmatrix}
\end{aligned} \tag{95}
$$

We can evaluate

$$
\begin{aligned}
\det\overline{\mathbf{g}}_1 &= \left(\rho_0-\rho_1\right)^6 \frac{9}{4}\frac{\left(1-\varepsilon_1^2\right)^{\frac{2}{3}}\left(1-\varepsilon_2^2\right)^{\frac{2}{3}}}{\varepsilon_1^2\varepsilon_2^2\left(\varepsilon_1^4+\varepsilon_2^4-\varepsilon_1^2\varepsilon_2^2\right)\left(\varepsilon_1^2-\varepsilon_2^2\right)^2} d_0 d_1 d_2 \\
&= \frac{\left(\rho_0-\rho_1\right)^6}{\rho_1}\frac{256}{2025}\pi^3 R^{20}\frac{\varepsilon_1^2\varepsilon_2^2\left(\varepsilon_1^2\varepsilon_2^2-2\varepsilon_1^2-2\varepsilon_2^2+3\right)}{\left(1-\varepsilon_1^2\right)^{\frac{8}{3}}\left(1-\varepsilon_2^2\right)^{\frac{8}{3}}} \\
&\times F_{01}\left(a_1\right)\frac{F_{21}\left(a_1\right)}{2a_1a_2a_3\left(\rho_0-\rho_1\right)F_{21}\left(a_1\right)+5\rho_1}\frac{F_{22}\left(a_1\right)}{2a_1a_2a_3\left(\rho_0-\rho_1\right)F_{22}\left(a_1\right)+5\rho_1}
\end{aligned} \tag{96}
$$

But

$$
\det\mathbf{V} = R^2\frac{\varepsilon_1\varepsilon_2}{\left(1-\varepsilon_1^2\right)\left(1-\varepsilon_2^2\right)} \tag{97}
$$

so

$$
\det\overline{\mathbf{g}}_1 = \left(\det\mathbf{V}\right)^2\frac{\left(\rho_0-\rho_1\right)^6}{\rho_1}\frac{256}{2025}\pi^3 R^{16}\frac{\left(\varepsilon_1^2\varepsilon_2^2-2\varepsilon_1^2-2\varepsilon_2^2+3\right)}{\left(1-\varepsilon_1^2\right)^{\frac{2}{3}}\left(1-\varepsilon_2^2\right)^{\frac{2}{3}}} \tag{98}
$$

Using the previous result,

$$\det \mathbf{g}_1 = \frac{256}{2025}\pi^3 \frac{(\rho_0-\rho_1)^6}{\rho_1} \frac{R^{16}}{(1-\varepsilon_1^2)^{\frac{2}{3}}(1-\varepsilon_2^2)^{\frac{2}{3}}} \left(\varepsilon_1^2\varepsilon_2^2 - 2\varepsilon_1^2 - 2\varepsilon_2^2 + 3\right) \times F_{01}(a_1) \frac{F_{21}(a_1)}{2a_1a_2a_3(\rho_0-\rho_1)F_{21}(a_1)+5\rho_1} \frac{F_{22}(a_1)}{2a_1a_2a_3(\rho_0-\rho_1)F_{22}(a_1)+5\rho_1} \tag{99}$$

which agrees.

A further convienient change of coordinates is

$$\begin{aligned} x_1 &= \varepsilon_1^2 \\ x_2 &= \varepsilon_2^2 \end{aligned} \tag{100}$$

In this case,

$$\mathbf{V}_a^i = \frac{\partial X^i}{\partial Y^a} = \begin{pmatrix} 1 & 0 & 0 \\ 0 & \frac{1}{2\varepsilon_1} & 0 \\ 0 & 0 & \frac{1}{2\varepsilon_2} \end{pmatrix} \tag{101}$$

so

$$\begin{aligned} \left(\overline{\overline{\mathbf{g}}}_1\right)_{11} &= (\rho_0-\rho_1)^2 R^4 d_0 \\ \left(\overline{\overline{\mathbf{g}}}_1\right)_{12} &= \left(\overline{\overline{\mathbf{g}}}_1\right)_{13} = \left(\overline{\overline{\mathbf{g}}}_1\right)_{21} = \left(\overline{\overline{\mathbf{g}}}_1\right)_{31} = 0 \\ \left(\overline{\overline{\mathbf{g}}}_1\right)_{22} &= (\rho_0-\rho_1)^2 \frac{1}{8R^4} \frac{(1-x_2)^{\frac{4}{3}}}{x_1^2(1-x_1)^{\frac{2}{3}}(x_1-x_2)^2(x_1^2-x_1x_2+x_2^2)} \begin{pmatrix} \left(5x_1^2+2x_2^2-5x_1x_2\right)(d_1+d_2) \\ -2(2x_1-x_2)(d_1-d_2)\sqrt{x_1^2+x_2^2-x_1x_2} \end{pmatrix} \\ \left(\overline{\overline{\mathbf{g}}}_1\right)_{23} &= \left(\overline{\overline{\mathbf{g}}}_1\right)_{32} = (\rho_0-\rho_1)^2 \frac{1}{8R^2} \frac{\sqrt[3]{1-x_1}\sqrt[3]{1-x_2}}{x_1x_2(x_1-x_2)^2(x_1^2-x_1x_2+x_2^2)} \begin{pmatrix} \left(x_1^2+x_2^2-4x_1x_2\right)(d_1+d_2) \\ +(x_1+x_2)\sqrt{x_1^2+x_2^2-x_1x_2}(d_1-d_2) \end{pmatrix} \\ \left(\overline{\overline{\mathbf{g}}}_1\right)_{33} &= (\rho_0-\rho_1)^2 \frac{1}{8R^2} \frac{(1-x_1)^{\frac{4}{3}}}{x_2^2(1-x_2)^{\frac{2}{3}}(x_1-x_2)^2(x_1^2-x_1x_2+x_2^2)} \begin{pmatrix} \left(2x_1^2+5x_2^2-5x_1x_2\right)(d_1+d_2) \\ +2\sqrt{x_1^2+x_2^2-x_1x_2}(x_1-2x_2)(d_1-d_2) \end{pmatrix} \end{aligned} \tag{102}$$

We can evaluate

$$\det \overline{\overline{\mathbf{g}}}_1 = \frac{(\rho_0-\rho_1)^6}{\rho_1} \frac{16}{2025}\pi^3 R^{20} \frac{x_1x_2-2x_1-2x_2+3}{(1-x_1)^{\frac{8}{3}}(1-x_2)^{\frac{8}{3}}} \times F_{01}(a_1) \frac{F_{21}(a_1)}{2R^3(\rho_0-\rho_1)F_{21}(a_1)+5\rho_1} \frac{F_{22}(a_1)}{2R^3(\rho_0-\rho_1)F_{22}(a_1)+5\rho_1} \tag{103}$$

### 1. *Weak Solution*

In the weak solution limit,

$$\begin{aligned} d_1+d_2 &= \left(\frac{\gamma_{21}\Lambda_1}{2a_1a_2a_3\rho_0}\right) + \left(\frac{\gamma_{22}\Lambda_2}{2a_1a_2a_3\rho_0}\right) \\ &= \frac{16}{1215}\pi \frac{R^7}{\rho_0(1-\varepsilon_1^2)^{\frac{5}{3}}(1-\varepsilon_2^2)^{\frac{5}{3}}} \left(\varepsilon_1^4 - \varepsilon_1^2\varepsilon_2^2 + \varepsilon_2^4\right)\left(-4\varepsilon_1^6 + 3\varepsilon_1^4\varepsilon_2^2 + 6\varepsilon_1^4 + 3\varepsilon_1^2\varepsilon_2^4 - 6\varepsilon_1^2\varepsilon_2^2 - 4\varepsilon_2^6 + 6\varepsilon_2^4\right) \\ d_1-d_2 &= \left(\frac{\gamma_{21}\Lambda_1}{2a_1a_2a_3\rho_0}\right) - \left(\frac{\gamma_{22}\Lambda_2}{2a_1a_2a_3\rho_0}\right) \\ &= -\frac{16}{1215}\pi R^7 \frac{6\varepsilon_1^6 + 6\varepsilon_2^6 - 4\varepsilon_1^8 - 4\varepsilon_2^8 - 9\varepsilon_1^2\varepsilon_2^4 - 9\varepsilon_1^4\varepsilon_2^2 + 5\varepsilon_1^2\varepsilon_2^6 + 5\varepsilon_1^6\varepsilon_2^2}{\rho_0\left(\sqrt[3]{1-\varepsilon_1^2}\right)^5\left(\sqrt[3]{1-\varepsilon_2^2}\right)^5} \sqrt{\varepsilon_1^4 - \varepsilon_1^2\varepsilon_2^2 + \varepsilon_2^4} \end{aligned} \tag{104}$$

and

$$\overline{\mathbf{g}}_1 = \frac{4\pi\rho_0 R^5}{135\left(1-\varepsilon_1^2\right)^{\frac{1}{3}}\left(1-\varepsilon_2^2\right)^{\frac{1}{3}}} \times \begin{pmatrix} \frac{135}{R}\frac{\rho_0}{\rho_1}\left(1-\varepsilon_1^2\right)^{\frac{1}{3}}\left(1-\varepsilon_2^2\right)^{\frac{1}{3}} F_{01}\left(a_1\right) & 0 & 0 \\ 0 & \frac{\varepsilon_1^2}{\left(1-\varepsilon_1^2\right)^2}\left(6-4\varepsilon_1^2-\varepsilon_2^2\right) & -\frac{\varepsilon_1\varepsilon_2}{\left(1-\varepsilon_1^2\right)\left(1-\varepsilon_2^2\right)}\left(3-2\varepsilon_1^2-2\varepsilon_2^2\right) \\ 0 & -\frac{\varepsilon_1\varepsilon_2}{\left(1-\varepsilon_1^2\right)\left(1-\varepsilon_2^2\right)}\left(3-2\varepsilon_1^2-2\varepsilon_2^2\right) & \frac{\varepsilon_2^2}{\left(1-\varepsilon_2^2\right)^2}\left(6-\varepsilon_1^2-4\varepsilon_2^2\right) \end{pmatrix} \tag{105}$$

*2. Small eccentricity expansion*

Small eccentricities gives

$$\begin{aligned} \overline{\overline{\mathbf{g}}}_{00} &= \frac{4\pi\left(\rho_0-\rho_1\right)^2}{\rho_1} R^3\left(1-\alpha^2\frac{1}{45}\left(x_1^2+x_2^2-x_1x_2\right)+O\left(\alpha^3\right)\right) \\ \overline{\overline{\mathbf{g}}}_{11} &= \frac{8\pi}{45}\frac{\left(\rho_0-\rho_1\right)^2}{2\rho_0+3\rho_1} R^5\left(1+\alpha\frac{1}{21}\frac{1}{2\rho_0+3\rho_1}\left(10\left(7\rho_0+12\rho_1\right)x_1+\left(7\rho_0+3\rho_1\right)x_2\right)+O\left(\alpha^2\right)\right) \\ \overline{\overline{\mathbf{g}}}_{12} &= -\frac{4\pi}{45}\frac{\left(\rho_0-\rho_1\right)^2}{2\rho_0+3\rho_1} R^5\left(1+\alpha\frac{1}{21}\frac{28\rho_0+57\rho_1}{2\rho_0+3\rho_1}\left(x_1+x_2\right)+O\left(\alpha^2\right)\right) \\ \overline{\overline{\mathbf{g}}}_{22} &= \frac{8\pi}{45}\frac{\left(\rho_0-\rho_1\right)^2}{2\rho_0+3\rho_1} R^5\left(1+\alpha\frac{1}{21}\frac{1}{2\rho_0+3\rho_1}\left(\left(7\rho_0+3\rho_1\right)x_1+10\left(7\rho_0+12\rho_1\right)x_2\right)+O\left(\alpha^2\right)\right) \end{aligned} \tag{106}$$

and

$$\det\overline{\overline{\mathbf{g}}} = \frac{\left(4\pi\left(\rho_0-\rho_1\right)^2\right)^3}{\rho_1\left(2\rho_0+3\rho_1\right)^2} R^{13}\frac{1}{675}\left[1+2\alpha\left(x_1+x_2\right)+O\left(\alpha^2\right)\right] \tag{107}$$

The free energy is

$$\beta F = \beta F_c$$

## Appendix A: Lame Functions

The only interior functions we need are

$$\begin{aligned} E_0^1\left(x\right) &= 1 \\ E_2^1\left(x\right) &= x^2+\Lambda_1-a_1^2 \\ E_2^2\left(x\right) &= x^2+\Lambda_2-a_1^2 \end{aligned} \tag{A1}$$

The exterior functions have the general definition

$$F_n^p\left(x\right) = \left(2n+1\right)E_n^p\left(x\right)I_n^p\left(x\right) = \left(2n+1\right)E_n^p\left(x\right)\int_x^\infty\left(\frac{1}{E_n^p\left(t\right)}\right)^2\frac{dt}{\sqrt{t^2-h_2^2}\sqrt{t^2-h_3^2}} \tag{A2}$$

so

$$\begin{aligned} F_n^p\left(a_1\right) &= \left(2n+1\right)E_n^p\left(a_1\right)\frac{1}{a_1}\int_1^\infty\left(\frac{1}{E_n^p\left(a_1y\right)}\right)^2\frac{dy}{\sqrt{y^2-\varepsilon_1^2}\sqrt{y^2-\varepsilon_2^2}} \\ &= \left(2n+1\right)E_n^p\left(a_1\right)\frac{1}{a_1}\int_0^1\left(\frac{1}{E_n^p\left(a_1/z\right)}\right)^2\frac{dz}{\sqrt{1-\varepsilon_1^2z^2}\sqrt{1-\varepsilon_2^2z^2}} \\ &= \left(2n+1\right)E_n^p\left(a_1\right)\frac{\left(1-\varepsilon_1^2\right)^{1/6}\left(1-\varepsilon_2^2\right)^{1/6}}{R\varepsilon_1}\int_0^{\arcsin\varepsilon_1}\left(\frac{1}{E_n^p\left(\frac{R}{\varepsilon_1\left(1-\varepsilon_1^2\right)^{1/6}\left(1-\varepsilon_2^2\right)^{1/6}\sin\theta}\right)}\right)^2\frac{d\theta}{\sqrt{1-\left(\frac{\varepsilon_2}{\varepsilon_1}\right)^2\left(\sin\theta\right)^2}} \end{aligned} \tag{A3}$$

Define

$$\phi = \arcsin \varepsilon_1 \qquad \text{(A4)}$$
$$\alpha = \arcsin \frac{\varepsilon_2}{\varepsilon_1}$$

Then, Dasios gives

$$I_0^1(x) = \frac{1}{h_2} F(\phi|\alpha) \qquad \text{(A5)}$$
$$I_2^j(x) = \frac{1}{2(\Lambda_j - a_1^2)(\Lambda_j - a_2^2)(\Lambda_j - a_3^2)} \left( h_2 E(\phi|\alpha) - \frac{\Lambda_j - a_3^2}{h_2} F(\phi|\alpha) \right)$$
$$+ \frac{1}{2x\sqrt{x^2 - h_2^2}\sqrt{x^2 - h_3^2}} \left( \frac{1}{x^2 + \Lambda_j - a_1^2} + \frac{1}{h_1^2} \frac{x^2 - h_2^2}{\Lambda_j - a_2^2} - \frac{1}{h_1^2} \frac{x^2 - h_3^2}{\Lambda_j - a_3^2} \right)$$

where the incomplete elliptic integrals are

$$E(\phi|\alpha) = \int_0^\phi \sqrt{1 - (\sin\alpha)^2 (\sin\theta)^2} d\theta \qquad \text{(A6)}$$
$$F(\phi|\alpha) = \int_0^\phi \frac{1}{\sqrt{1 - (\sin\alpha)^2 (\sin\theta)^2}} d\theta$$

Thus

$$F_0^1(a_1) = \frac{1}{a_1} \int_1^\infty \frac{dy}{\sqrt{y^2 - \varepsilon_1^2}\sqrt{y^2 - \varepsilon_2^2}}$$

### Appendix B: Expansion for small eccentricites

In general

$$a_1 = \frac{R}{(1 - \alpha\varepsilon_1^2)^{1/6} (1 - \alpha\varepsilon_2^2)^{1/6}} \qquad \text{(B1)}$$
$$a_2 = \frac{R}{(1 - \alpha\varepsilon_1^2)^{1/6} (1 - \alpha\varepsilon_2^2)^{1/6}} \left(1 - \alpha\varepsilon_1^2\right)^{1/2}$$
$$a_3 = \frac{R}{(1 - \alpha\varepsilon_1^2)^{1/6} (1 - \alpha\varepsilon_2^2)^{1/6}} \left(1 - \alpha\varepsilon_2^2\right)^{1/2}$$

and

$$h_2^2 = a_1^2 - a_3^2 = \varepsilon_2^2 \frac{R^2}{(1 - \varepsilon_1^2)^{1/3} (1 - \varepsilon_2^2)^{1/3}} = R^2 \varepsilon_2^2 \left(1 + O\left(\varepsilon_1^2, \varepsilon_2^2\right)\right) \qquad \text{(B2)}$$
$$h_3^2 = a_1^2 - a_2^2 = \varepsilon_1^2 \frac{R^2}{(1 - \varepsilon_1^2)^{1/3} (1 - \varepsilon_2^2)^{1/3}} = R^2 \varepsilon_1^2 \left(1 + O\left(\varepsilon_1^2, \varepsilon_2^2\right)\right)$$

Also

$$\Lambda_1 = \frac{1}{3} \frac{R^2}{\sqrt[3]{1 - \alpha\varepsilon_1^2}\sqrt[3]{1 - \alpha\varepsilon_2^2}} \left( -\left(\alpha\varepsilon_1^2 + \alpha\varepsilon_2^2 - 3\right) + \alpha\sqrt{\left(\varepsilon_1^4 - \varepsilon_1^2\varepsilon_2^2 + \varepsilon_2^4\right)} \right) \qquad \text{(B3)}$$
$$\Lambda_2 = \frac{1}{3} \frac{R^2}{\sqrt[3]{1 - \alpha\varepsilon_1^2}\sqrt[3]{1 - \alpha\varepsilon_2^2}} \left( -\left(\alpha\varepsilon_1^2 + \alpha\varepsilon_2^2 - 3\right) - \alpha\sqrt{\left(\varepsilon_1^4 - \varepsilon_1^2\varepsilon_2^2 + \varepsilon_2^4\right)} \right)$$

So

$$F_0^1\left(a_1\right)=\frac{1}{a_1}\int_1^{\infty}\frac{dy}{\sqrt{y^2-\varepsilon_2^2}\sqrt{y^2-\varepsilon_1^2}} \tag{B4}$$
$$=\frac{1}{a_1}\left(1+\alpha\frac{1}{6}\left(\varepsilon_1^2+\varepsilon_2^2\right)+\alpha^2\frac{1}{40}\left(3\varepsilon_1^4+3\varepsilon_2^4+2\varepsilon_1^2\varepsilon_2^2\right)+O\left(\alpha^3\right)\right)$$
$$=\frac{1}{R}\left(1-\frac{1}{45}\alpha^2\left(\varepsilon_1^4-\varepsilon_1^2\varepsilon_2^2+\varepsilon_2^4\right)+O\left(\alpha^3\right)\right)$$

Similarly

$$F_2^p\left(a_1\right)=5\Lambda_j\frac{1}{a_1}\int_1^{\infty}\left(\frac{1}{a_1^2y^2+\Lambda_j-a_1^2}\right)^2\frac{dy}{\sqrt{y^2-\varepsilon_1^2}\sqrt{y^2-\varepsilon_2^2}} \tag{B5}$$

giving

$$F_2^1\left(a_1\right)=\frac{1}{R^3}\left(1-\alpha\frac{1}{7}\sqrt{\varepsilon_1^4-\varepsilon_1^2\varepsilon_2^2+\varepsilon_2^4}-\alpha^2\frac{1}{21}\left(\varepsilon_1^4+\varepsilon_2^4-\varepsilon_1^2\varepsilon_2^2+\left(\varepsilon_1^2+\varepsilon_2^2\right)\sqrt{\varepsilon_1^4-\varepsilon_1^2\varepsilon_2^2+\varepsilon_2^4}\right)+O\left(\alpha^3\right)\right) \tag{B6}$$
$$F_2^2\left(a_1\right)=\frac{1}{R^3}\left(1+\alpha\frac{1}{7}\sqrt{\varepsilon_1^4-\varepsilon_1^2\varepsilon_2^2+\varepsilon_2^4}-\alpha^2\frac{1}{21}\left(\varepsilon_1^4+\varepsilon_2^4-\varepsilon_1^2\varepsilon_2^2-\left(\varepsilon_1^2+\varepsilon_2^2\right)\sqrt{\varepsilon_1^4-\varepsilon_1^2\varepsilon_2^2+\varepsilon_2^4}\right)+O\left(\alpha^3\right)\right)$$

So

$$\gamma\mathcal{F}\left(a_1\right)\left[a_2a_3\left(\rho_0-\rho_1\right)\left(\frac{d}{d\xi}\mathcal{E}\left(\xi\right)\right)\mathcal{F}\left(a_1\right)+\rho_1\mathcal{W}\right]^{-1}\mathcal{E}\left(a_1\right) \tag{B7}$$
$$=4\pi\,\mathrm{diag}\begin{pmatrix}\frac{F_0^1(a_1)}{\rho_1},\\ -\frac{2}{5}\left(\Lambda_1-\Lambda_2\right)\left(\Lambda_1-a_1^2\right)\left(\Lambda_1-a_2^2\right)\left(\Lambda_1-a_3^2\right)\frac{F_2^1(a_1)}{2a_1a_2a_3(\rho_0-\rho_1)F_2^1(a_1)+5\rho_1}\Lambda_1,\\ \frac{2}{5}\left(\Lambda_1-\Lambda_2\right)\left(\Lambda_2-a_1^2\right)\left(\Lambda_2-a_2^2\right)\left(\Lambda_2-a_3^2\right)\frac{F_2^2(a_1)}{2a_1a_2a_3(\rho_0-\rho_1)F_2^2(a_1)+5\rho_2}\Lambda_2\end{pmatrix}$$

where "diag" means the diagonal matrix with these entries.

Taking out a factor $\frac{4\pi}{\rho_1}$ the diagonal elements are

$$D_{00}=\frac{1}{R}\left(1-\frac{1}{45}\alpha^2\left(x_1^2+x_2^2-x_1x_2\right)+O\left(\alpha^3\right)\right)$$
$$D_{11}+D_{22}=\alpha^4R^7\begin{bmatrix}\frac{16}{405}\frac{\rho_1}{2\rho_0+3\rho_1}\left(x_1^2-x_1x_2+x_2^2\right)^2\\ +\alpha\frac{16}{2835}\frac{\rho_1}{(2\rho_0+3\rho_1)^2}\left(x_1^3+x_2^3\right)\left(14x_1^2\rho_0+26x_1^2\rho_1+14x_2^2\rho_0+26x_2^2\rho_1-7x_1x_2\rho_0-23x_1x_2\rho_1\right)+O\left(\alpha^2\right)\end{bmatrix}$$
$$D_{11}-D_{22}=\alpha^4R^7\frac{8}{405}\sqrt{x_1^2-x_1x_2+x_2^2}$$
$$\times\begin{bmatrix}-\frac{\rho_1}{2\rho_0+3\rho_1}\left(2x_1^3-3x_1^2x_2-3x_1x_2^2+2x_2^3\right)\\ -\frac{2}{21}\alpha\frac{\rho_1}{(2\rho_0+3\rho_1)^2}\left(42x_1^4\rho_0+78x_1^4\rho_1+42x_2^4\rho_0+78x_2^4\rho_1-210x_1^2x_2^2\rho_0-30x_1x_2^3\rho_1-270x_1^2x_2^2\rho_1-30x_1^3x_2\rho_1\right)\\ +O\left(\alpha^2\right)\end{bmatrix}$$

Then from the general expression

$$\overline{\overline{\mathbf{g}}}_1=\left(\rho_0-\rho_1\right)^2R^6\frac{4\pi}{\rho_1}$$
$$\times\begin{pmatrix}\frac{1}{R^2}D_{00} & 0 & \\ 0 & \frac{1}{8R^8}\frac{(1-x_2)^{\frac{4}{3}}}{x_1^2(1-x_1)^{\frac{2}{3}}(x_1-x_2)^2\left(x_1^2-x_1x_2+x_2^2\right)}\begin{pmatrix}\left(5x_1^2+2x_2^2-5x_1x_2\right)\left(D_{11}+D_{22}\right)\\ -2\left(2x_1-x_2\right)\left(D_{11}-D_{22}\right)\sqrt{x_1^2+x_2^2-x_1x_2}\end{pmatrix} & \frac{1}{8R^8}\frac{\sqrt[3]{1-x_1}\,\sqrt[3]{1-x_2}}{x_1x_2(x_1-x_2)^2\left(x_1^2-x_1x_2+\text{[illegible]}\right.}\text{[illegible]} \\ 0 & \frac{1}{8R^8}\frac{\sqrt[3]{1-x_1}\,\sqrt[3]{1-x_2}}{x_1x_2(x_1-x_2)^2\left(x_1^2-x_1x_2+x_2^2\right)}\begin{pmatrix}\left(x_1^2+x_2^2-4x_1x_2\right)\left(D_{11}+D_{22}\right)\\ +\left(x_1+x_2\right)\sqrt{x_1^2+x_2^2-x_1x_2}\left(D_{11}-D_{22}\right)\end{pmatrix} & \frac{1}{8R^8}\frac{(1-x_1)^{\frac{4}{3}}}{x_2^2(1-x_2)^{\frac{2}{3}}(x_1-x_2)^2\left(x_1^2-x_1x_2\text{[illegible]}\right.}\text{[illegible]}\end{pmatrix}$$

we get

$$\bar{\bar{\mathbf{g}}}_{00} = \frac{4\pi\left(\rho_0-\rho_1\right)^2}{\rho_1} R^3\left(1-\alpha^2 \frac{1}{45}\left(x_1^2+x_2^2-x_1 x_2\right)+O\left(\alpha^3\right)\right) \tag{B8}$$

$$\bar{\bar{\mathbf{g}}}_{11} = \frac{8\pi}{45} \frac{\left(\rho_0-\rho_1\right)^2}{2\rho_0+3\rho_1} R^5\left(1+\alpha \frac{1}{21} \frac{1}{2\rho_0+3\rho_1}\left(10\left(7\rho_0+12\rho_1\right) x_1+\left(7\rho_0+3\rho_1\right) x_2\right)+O\left(\alpha^2\right)\right)$$

$$\bar{\bar{\mathbf{g}}}_{12} = -\frac{4\pi}{45} \frac{\left(\rho_0-\rho_1\right)^2}{2\rho_0+3\rho_1} R^5\left(1+\alpha \frac{1}{21} \frac{28\rho_0+57\rho_1}{2\rho_0+3\rho_1}\left(x_1+x_2\right)+O\left(\alpha^2\right)\right)$$

$$\bar{\bar{\mathbf{g}}}_{22} = \frac{8\pi}{45} \frac{\left(\rho_0-\rho_1\right)^2}{2\rho_0+3\rho_1} R^5\left(1+\alpha \frac{1}{21} \frac{1}{2\rho_0+3\rho_1}\left(\left(7\rho_0+3\rho_1\right) x_1+10\left(7\rho_0+12\rho_1\right) x_2\right)+O\left(\alpha^2\right)\right)$$

and

$$\det \bar{\bar{\mathbf{g}}} = \frac{\left(4\pi\left(\rho_0-\rho_1\right)^2\right)^3}{\rho_1\left(2\rho_0+3\rho_1\right)^2} R^{13} \frac{1}{675}\left[1+2\alpha\left(x_1+x_2\right)+O\left(\alpha^2\right)\right] \tag{B9}$$

For $\rho_0 \gg \rho_1$, these are approximately

$$\bar{\bar{\mathbf{g}}}_{00} = \frac{4\pi\rho_0^2}{\rho_1} R^3\left(1-\alpha^2 \frac{1}{45}\left(x_1^2+x_2^2-x_1 x_2\right)+O\left(\alpha^3\right)\right) \tag{B10}$$

$$\bar{\bar{\mathbf{g}}}_{11} = \frac{4\pi}{45} \rho_0 R^5\left(1+\alpha \frac{1}{6}\left(10 x_1+x_2\right)+O\left(\alpha^2\right)\right)$$

$$\bar{\bar{\mathbf{g}}}_{12} = -\frac{2\pi}{45} \rho_0 R^5\left(1+\alpha \frac{2}{3}\left(x_1+x_2\right)+O\left(\alpha^2\right)\right)$$

$$\bar{\bar{\mathbf{g}}}_{22} = \frac{4\pi}{45} \rho_0 R^5\left(1+\alpha \frac{1}{6}\left(x_1+10 x_2\right)+O\left(\alpha^2\right)\right)$$

and

$$\det \bar{\bar{\mathbf{g}}} = \frac{16\pi^3}{675} \frac{\rho_0^4}{\rho_1} R^{13}\left[1+2\alpha\left(x_1+x_2\right)+O\left(\alpha^2\right)\right] \tag{B11}$$
